# Supplementary material for: On (Omega-)Regular Model Checking
Source: arXiv:0809.2214 source file (2008-09-12)
Supplement: Supplementary file 1 [file appendix.tex]

\newpage
\section*{Appendix. Proofs of Theorems of Section \ref{extrap-1}}
\label{app1}

Proof of Theorem \ref{th-algo-count1}

\begin{proof} 
We make the distinction between the finite and the infinite word
cases.
\begin{itemize}
\item
We start with the finite word case, and show that for each $w_c =
(w(1),c_1)(w(2),c_2)$\\${\dots}(w(n),c_n)$ $\in$ $L(A^{e_*}_c)$ with
$P(w_c) = (w,i)$, we have $w$ $\in$ $L(A^{e_i})$. The result is
immediate if $i = 0$. We now suppose $i>0$. Consider the unique
accepting run $\pi^{e_*} =
q_0^{e_*}q_1^{e_*}q_2^{e_*}{\dots}q_n^{e_*}$ on $w_c\in
L(A^{e_*}_c)$. We show that there exists an accepting run $\pi^{e_i} =
q_0^{e_i}q_1^{e_i}q_2^{e_i}{\dots}q_n^{e_i}$ on the word $w\in
L(A^{e_i})$. This is done by associating a state of $A^{e_i}$ to each
state of $\pi^{e_*}$.

Let $q_0^{e_*}q_1^{e_*}q_2^{e_*}{\dots}q_u^{e_*}$ be the part of
$\pi^{e_*}$ that stays in $Q_H^{e_*}$. Since $Q_H^{e_*}$ and
$Q_H^{e_i}$ are isomorphic, the corresponding states in $A^{e_i}$ are
$q_0^{e_i},q_1^{e_i},q_2^{e_i},{\dots},q_u^{e_i}$, where $q_j^{e_i}\in
Q_H^{e_i}$ is isomorphic to $q_j^{e_*}$, $\forall{j}$ $\in$
${\lbrack}0{\dots}u{\rbrack}$. If $ q^{e_*}_{u+1} =
\delta(q_u^{e_*},(w(u+1),c_{u+1}=i))$ and $q^{e_*}_{u+1}$ $\in$
$Q_{I_{j{\geq}1}}^{e_*}$ then, since $A^{e_0}$ and $A^{e_i}$ are
communication stable, there exists $q^{e_i}_{u+1}\in
Q_{I_{j+i}}^{e_i}$ such that $q^{e_i}_{u+1} =
\delta(q_u^{e_i},w(u+1))$. This state is the state corresponding to
$q^{e_*}_{u+1}$ by the increment isomorphism. By definition there
exists a forward equivalence between $Q_{I_{j+i}}^{e_i}$ and
$Q_{I_{j{\geq}1}}^{e_0}$, and the result holds.

If $ q^{e_*}_{u+1} = \delta(q_u^{e_*},(w(u+1),c_{u+1}))$ and
$q^{e_*}_{u+1}$ $\in$ $Q_{I_0}^{e_*}$ then, since $A^{e_0}$ and
$A^{e_i}$ are communication stable, there exists $q^{e_i}_{u+1}\in
Q_{I_{c_{u+1}}}^{e_i}$ and $q^{e_i}_{u+1} =
\delta(q_u^{e_i},w(u+1))$. This state is the state corresponding to
$q_{u+1}^{e_*}$ by the increment isomorphism. Consider the part of
$\pi^{e_*}$ that stay in $Q_{I_0}^{e_*}$, and two states $q^{e_*}_{l
{\geq} u+1}$, $q^{e_*}_{l+1}$ with $q^{e_*}_{l+1} =
\delta(q^{e_*}_{l},(w(l+1),c_{l+1}))$. Let $q^{e_i}_{l}$ $\in$
$Q^{e_i}_{I_{z}}$ be the state corresponding to $q^{e_*}_{l}$ in
$\pi^{e_i}$ by the increment isomorphism, and $z = \sum_{k = 1}^{k =
l}c_k$. The state corresponding to $q^{e_*}_{l+1}$ in $\pi^{e_i}$ is
the state isomorphic to $q^{e_*}_{l+1}$ in
$Q_{I_{z+c_{l+1}}}^{e_i}$. If $c_{l+1}=0$, it is immediate. Otherwise, this
follows because of the transition
$(q^{e_*}_{l},(w(l+1),c_{l+1}),q^{e_*}_{l+1})$ that simulates the
existence of $c_{l+1}$ increments communication equivalent to
$Q_{I_0}^{e_0}$ and to $Q_{I_z}^{e_i}$. Let $q_k^{e_*}$ be the last
state of $\pi^{e_*}$ that belong to $Q_{I_0}^{e_*}$, and $q_k^{e_i}$
its corresponding state in $\pi^{e_i}$. If $q_k^{e_*}=q_n^{e_*}$, then
the result holds.

Otherwise, we have
$q^{e_*}_{k+1}=\delta^{e_*}(q_k^{e_*},(w(k+1),c_{k+1}))$. If $c_{k+1} =
0$, then $q_k^{e_i}$ $\in$ $Q_{I_{i}}^{e_i}$ . There exists a forward
equivalence between states of $Q_{I_{i}}^{e_i}$ and of
$Q_{I_{0}}^{e_0}$, and the result holds. If $c_{k+1} > 0$, then
$q_k^{e_i}$ $\in$ $Q_{I_{i-{c_{k+1}}}}^{e_i}$ and $q_{k+1}^{e_*}$
$\in$ $Q_{I_{m > 0}}^{e_*}$. Due to the communication equivalence
property, there exists
$q^{e_i}_{k+1}=\delta^{e_i}(q_{k}^{e_i},w(k+1))$ and $q^{e_i}_{k+1}$
$\in$ $Q_{i+m}^{e_i}$. This state is the state corresponding to
$q^{e_*}_{k+1}$ by the increment isomorphism. Since states of
$Q_{I_{i+m}}^{e_i}$ and of $Q_{I_{m}}^{e_0}$ are in forward
equivalence, the result holds.
\item
We now consider the infinite word case, and show that for each $w_c =
(w(1),c_1)$\\$(w(2),c_2){\dots}(w(n),c_n)(\Sigma,0)^{\omega}$ $\in$
$L(A^{e_*}_c)$ with $P(w_c) = (w,i)$, there exists $w$ $\in$
$L(A^{e_i})$. The result is immediate if $i = 0$. We now suppose
$i>0$. Consider the unique accepting run $\pi^{e_*} =
q_0^{e_*}q_1^{e_*}q_2^{e_*}{\dots}q_n^{e_*}({sc}^{e_*})^{\omega}$ on
the word $w_c$ in $A^{e_*}_c$. We show that there exists an accepting
run $\pi^{e_i} =
q_0^{e_i}q_1^{e_i}q_2^{e_i}{\dots}q_n^{e_i}(sc^{e_i})^{\omega}$ on the
word $w$ in $A^{e_i}$. Let
$q_0^{e_*}q_1^{e_*}q_2^{e_*}{\dots}q_u^{e_*}$ be the part of
$\pi^{e_*}$ that stays in $Q_H^{e_*}$. Since $Q_H^{e_*}$ and
$Q_H^{e_i}$ are isomorphic, the corresponding states in $A^{e_i}$ are
$q_0^{e_i},q_1^{e_i},q_2^{e_i},{\dots},q_u^{e_i}$, where $q_j^{e_i}\in
Q_H^{e_i}$ is isomorph to $q_j^{e_*}$, $\forall{j}$ $\in$
${\lbrack}0{\dots}u{\rbrack}$. If $q^{e_*}_{u+1} =
\delta(q_u^{e_*},(w(u+1),i))$, and $q^{e_*}_{u+1}$ $\in$
$Q_{I_{j{\geq}1}}^{e_*}$ then, since $A^{e_0}$ and $A^{e_i}$ are
communication stable, there exists $q^{e_i}_{u+1}\in
Q_{I_{j+i}}^{e_i}$, such that $q^{e_i}_{u+1} =
\delta(q_u^{e_i},w(u+1))$ is the state corresponding to $q^{e_*}_u$ by
the increment isomorphism. By definition there exists a forward
equivalence between $Q_{I_{j+i}}^{e_i}$ and $Q_{I_{j{\geq}1}}^{e_0}$,
and the result holds. Otherwise, we have to consider two situations.

\begin{enumerate}
\item

If $ q^{e_*}_{u+1} = \delta(q_u^{e_*},(w(u+1),0))$ and $q^{e_*}_{u+1}$
$\in$ $Q_{I_0}^{e_*}$ then, since $A^{e_0}$ and $A^{e_i}$ are
communication stable, there exists $q^{e_i}_{u+1}\in Q_{I_{0}}^{e_i}$
such that $q^{e_i}_{u+1} = \delta(q_u^{e_i},w(u+1))$ is the state
corresponding to $q_{u+1}^{e_*}$ by the increment isomorphism. Assume
that $sc^{e_*}~{\not\subseteq}~Q_{I_0}^{e_*}$. Let
$q_{u+1}^{e_*}{\dots}q_{u+k}^{e_*}$ the part of $\pi^{e_*}$ that stays
in $Q_{I_0}^{e_*}$.  Since $Q_{I_0}^{e_*}$ and $Q_{I_0}^{e_i}$ are
isomorphic, their exists corresponding states
$q_{u+1}^{e_i},{\dots},q_{u+k}^{e_i}$ in $Q_{I_0}^{e_i}$. Consider the
state $q_{u+k+1} = \delta^{e_*}(q_{u+k},(w(u+k+1)))$, and
assume that $q_{u+k+1}$ $\not\in$ $Q^{e_*}_{I_0}$. We have two situations.

First, $q^{e_*}_{u+k+1}$ $\in$ $Q_{I_{j{\geq}1}}^{e_*}$. In that case,
$c_{u+k+1}=i$. Since $A^{e_0}$ and $A^{e_i}$ are communication
equivalent, there exists $q^{e_i}_{u+k+1}\in Q_{I_{j+i}}^{e_i}$ such
that $q^{e_i}_{u+k+1} = \delta(q_u^{e_i},w(u+k+1))$ is the state
corresponding to $q^{e_*}_{u+k+1}$ by the increment isomorphism. There
exists a forward equivalence between $Q_{I_{i}}^{e_i}$ and
$Q_{I_{j{\geq}1}}^{e_0}$, and the results holds

Second, $q^{e_*}_{u+k+1}$ $\in$ $Q_{I_{0}COPY}^{e_*}$. Since
$A^{e_0}$ and $A^{e_i}$ are communication equivalent, there must
exists a state $q^{e_i}_{u+k+1}\in Q_{I_{c_{u+k+1}}}^{e_i}$ such that
$q^{e_i}_{u+k+1} =
\delta(q_{u+k}^{e_i},w(u+k+1))$. This state is the state corresponding
to $q_{u+k+1}^{e_*}$ by the increment isomorphism. The rest of this
case in treated in the next point.
 
\item

If $q^{e_*}_{u+1}$ $\in$ $Q_{I_{0}COPY}^{e_*}$ then, since $A^{e_0}$
and $A^{e_i}$ are communication stable, there exists $q^{e_i}_{u+1}\in
Q_{I_{c_{u+1}}}^{e_i}$ such that $q^{e_i}_{u+1} =
\delta(q_{u}^{e_i},w(u+1))$ is the state corresponding to
$q^{e_*}_u$ by the increment isomorphism. Consider the part of
$\pi^{e_*}$ that stay in $Q_{I_{0}COPY}^{e_*}$ and two states
$q^{e_*}_{l {\geq} u+k+1}$, $q^{e_*}_{l+1}$ with $q^{e_*}_{l+1} =
\delta(q^{e_*}_{l},(w(l+1),c_{l+1}))$. Let $q^{e_i}_{l}$ $\in$
$Q^{e_i}_{I_{z}}$ be the state corresponding to $q^{e_i}_{l}$ in
$\pi^{e_i}$, where $z = \sum_{k = 1}^{k = l}c_k$. The state
corresponding to $q^{e_*}_{l+1}$ in $\pi^{e_i}$ is the state that is
isomorphic to $q^{e_*}_{l+1}$ in $Q_{I_{z+c_{l+1}}}^{e_i}$ by the
increment isomorphism. This is obvious if $c_{l+1}=0$, else it follows
from the fact that the transition
$(q^{e_*}_{l},(w(l+1),c_{l+1}),q^{e_*}_{l+1})$ simulates the existence
of $c_{l+1}$ increments that are communication equivalent to
$Q_{I_{0}COPY}^{e_*}$ and to $Q_{I_z}^{e_i}$.  Let $q_k^{e_*}$ be the
last state of $\pi^{e_*}$ that belongs to $Q_{I_{0}COPY}^{e_*}$ and
$q_k^{e_i}$ its corresponding state in $\pi^{e_i}$. Consider the
transition $(q^{e_*}_{k},(w(k+1),c_{k+1}),q^{e_*}_{k+1})$. If $c_{k+1}
= 0$, then $q_k^{e_i}$ $\in$ $Q_{I_{i}}^{e_i}$ . Since there exists a
forward equivalence between states of $Q_{I_{i}}^{e_i}$ and
$Q_{I_{0}}^{e_0}$, and by construction, the result follows. If
$c_{k+1} > 0$, then $q_k^{e_i}$ $\in$ $Q_{I_{i-{c_{k+1}}}}^{e_i}$ and
$q_{k+1}^{e_*}$ $\in$ $Q_{I_{m > 0}}^{e_*}$. Because of the
communication equivalence property, there exists a transition
$(q^{e_i}_{k},w(k+1),q^{e_i}_{k+1})$, where $q^{e_i}_{k+1}$ $\in$
$Q_{i+m}^{e_i}$ is the state corresponding to $q^{e_*}_{k+1}$ in
$\pi^{e_i}$. Since there exists a forward equivalence between states
of $Q_{I_{i+m}}^{e_i}$ and of $Q_{I_{m}}^{e_0}$, the result holds.
\end{enumerate}
\end{itemize}
\end{proof}

Proof of Theorem \ref{th-algo-count2}.

\begin{proof}
We make the distinction between the finite and the infinite word
cases.
\begin{itemize}
\item
We start with the finite word case, and show that for each
$i~{\geq}~0$, $w=w(1){\dots}w(n)$ $\in$ $L(A^{e_i})$, there exists
$w_c\in L(A_c^{e_*})$ such that $P(w_c) = (w,b)$, and
$b~{\leq}~i$. The result is immediate if $i = 0$. We now suppose
$i>0$. Consider the unique accepting run $\pi^{e_i} =
q_0^{e_i}q_1^{e_i}q_2^{e_i}{\dots}q_n^{e_i}$ on $w$ in $A^{e_i}_c$. We
show that there exists an accepting run $\pi^{e_*} =
q_0^{e_*}q_1^{e_*}q_2^{e_*}{\dots}q_n^{e_*}$ on $w_c$ in $A^{e_*}$.

Let $q_0^{e_i}q_1^{e_i}q_2^{e_i}{\dots}q_u^{e_i}$ be the part of the
run that stay in $Q_H^{e_i}$. Since $Q_H^{e_i}$ and $Q_{H}^{e_0}$ are
isomorphic, the corresponding states in $A^{e_*}$ are
$q_0^{e_*},q_1^{e_*},q_2^{e_*},{\dots},q_u^{e_*}$ where, for each $j$
$\in$ ${\lbrack}0{\dots}i{\rbrack}$, $q_j^{e_i}$ and $q_j^{e_*}$ are
the corresponding states by the isomorphism relation. If $q^{e_*}_u =
q^{e_*}_n$ or if the state that follows $q_u^{e_i}$ is a state of
$Q_{T_f}^{e_i}$, then the result holds.

Now, assume that $q^{e_i}_{u+1} = \delta(q^{e_u}_{i},w(u+1))$ and
$q^{e_i}_{u+1}$ $\in$ $Q_{I_{l{\geq}i}}^{e_i}$. Since $Q_H^{e_0}$ and
$Q_H^{e_i}$ are communication stable, their exists by construction
$q_{u+1}^{e_*}=\delta^{e_*}(q^{e_*}_u,(w(u+1),i))$, where
$q^{e_*}_{u+1}\in Q_{l-i}^{e_*}$. This state is the state
corresponding to $q_{u+1}^{e_i}$ by the increment isomorphism. By
definition there exists a forward equivalence between
$Q_{I_{l}}^{e_i}$ and $Q_{I_{l-i}}^{e_0}$, and the result holds.

Suppose that $q^{e_i}_{u+1} = \delta(q^{e_i}_{u},w(u+1))$, and
$q^{e_i}_{u+1}$ $\in$ $Q_{I_{c < i}}^{e_i}$. Since $Q_H^{e_0}$ and
$Q_H^{e_i}$ are communication stable, their exists a transition
$(q_{u}^{e_*},(w(u+1),c),q_{u+1}^{e_*})$, where $q^{e_*}_{u+1}\in
Q_{I_0}^{e_*}$ is the state corresponding to $q_{u+1}^{e_i}$ by the
increment isomorphism. Consider now the part of $\pi^{e_i}$ that stays
in $\cup_{b=c}^{b=i-1}Q^{e_i}_{I_b}$.  Takes two states $q^{e_i}_{l}$
$\in$ $Q_{I_{l}}^{e_i}$ and $q^{e_i}_{l+1}$ $\in$ $Q_{I_{l+u}}^{e_i}$
such that $q^{e_i}_{l+1} = \delta(q^{e_i}_{l},w(l+1))$, and let
$q^{e_*}_{l}$ $\in$ $Q^{e_*}_{I_{0}}$ be the corresponding state of
$q^{e_i}_{l}$ $\in$ $\pi^{e_*}$. By construction,
there exists a transition $(q_l^{e_*},(w(l+1),u),q_{l+1}^{e_*})$ with
$q_{l+1}^{e_*}\in Q_{I_0}^{e_*}$ and $q_{l+1}^{e_*}$ is the state
corresponding to $q_{l+1}^{e_i}$ by the increment isomorphism. Let
$q_k^{e_i}$ $\in$ $Q_{I_{z<i}}^{e_i}$ be the last state of $\pi^{e_i}$
in $\cup_{b=c}^{b=i-1}Q^{e_i}_{I_b}$, and $q_k^{e_*}$ its isomorphic
state in $Q_{I_{0}}^{e_*}$. Let
$(w(1),c_1)(w(2),c_2){\dots}(w(k),c_k)$ be the part of $w_c$ that have
been read between $q_0^{e_*}$ and $q_k^{e_*}$.  We pose $s = \sum_{i =
1}^{i=k}c_k $; it is easy to see that $s = z$. If $q_k^{e_i} =
q_n^{e_i}$ or $q_{k+1}^{e_i}$ $\in$ $Q_{T_f}^{e_i}$, then the result
holds. Otherwise, there exists a transition
$(q^{e_i}_k,(w(k+1),q_{k+1}^{e_i})$ with $q_{k+1}$ $\in$
$Q_{I_{i+l}}^{e_i}$. By construction, there exists a transition
$(q^{e_*}_{k},(w(k+1),i-z),q^{e_*}_{k+1}$ with $q^{e_*}_{k+1}$ the
state isomorphic to $q^{e_i}_k$ in $Q_{I_{l}}^{e_0}$. Due to the
forward equivalence between $Q_{I_{i+l}}^{e_i}$ and $Q_{I_{l}}^{e_0}$,
the result holds.
\item
We now consider the infinite word case, and show that for each
$i~{\geq}~0$, $w=w(1){\dots}w(n)\Sigma^{\omega}$ $\in$
$\Sigma^{\omega}$, if $w$ $\in$ $L(A^{e_i})$, then there exists
$w_c\in L(A_c^{e_*})$ such that $P(w_c) = (w,b)$, and
$b~{\leq}~i$. The result is immediate if $i = 0$. We now suppose that
$i$ is greater than $0$. Consider the unique accepting run $\pi^{e_i}
= q_0^{e_i}q_1^{e_i}q_2^{e_i}{\dots}q_n^{e_i}(sc^{e_i})^{\omega}$ on
$w$ in $A^{e_i}_c$. We show that there exists an accepting run
$\pi^{e_*} =
q_0^{e_*}q_1^{e_*}q_2^{e_*}{\dots}q_n^{e_*}$\\$(sc^{e_*})^{\omega}$ on
$w_c$ in $A^{e_*}$.

Let $q_0^{e_i}q_1^{e_i}q_2^{e_i}{\dots}q_u^{e_i}$ be the part of the
run that stay in $Q_H^{e_i}$. Since $Q_H^{e_i}$ and $Q_{H}^{e_0}$ are
isomorphic, the corresponding states in $A^{e_*}$ are
$q_0^{e_*},q_1^{e_*},q_2^{e_*},{\dots},q_u^{e_*}$, where for each $j$
$\in$ ${\lbrack}0{\dots}i{\rbrack}$, $q_j^{e_i}$ and $q_j^{e_*}$ are
the corresponding states by the isomorphism relation. If $q^{e_*}_u =
q^{e_*}_n$ or if the state that follows $q_u^{e_i}$ is a state of
$Q_{T_f}^{e_i}$, then the result holds.

Now, assume that $q^{e_i}_{u+1} = \delta(q^{e_i}_{u},w(u+1))$,
$q^{e_i}_{u+1}$ $\in$ $Q_{I_{l{\geq}i}}^{e_i}$. Since $Q_H^{e_0}$ and
$Q_H^{e_i}$ are communication stable, their exists by construction
$q_{u+1}^{e_*}=\delta^{e_*}(q_{u}^{e_*},(w(u+1),i))$, where
$q^{e_*}_{u+1}\in Q^{e_*}_{l-i}$ is the state corresponding to
$q_{u+1}^{e_i}$ by the increment isomorphism. By definition there
exists a forward equivalence between $Q_{I_{l}}^{e_i}$ and
$Q_{I_{l-i}}^{e_0}$, and the result follows.

If $q^{e_i}_{u+1} = \delta(w(u+1),q^{e_i}_{u})$ and that
$q^{e_i}_{u+1}$ $\in$ $Q_{I_{c < i}}^{e_i}$ then, since $Q_H^{e_0}$
and $Q_H^{e_i}$ are communication stable, their exists
$q_{u+1}^{e_*}=\delta^{e_*}(q_{u}^{e_*},(w(u+1),c))$, and
$q^{e_*}_{u+1}\in Q_{I_{0}COPY}^{e_*}$. This state is the state
corresponding to $q_{u+1}^{e_i}$ by the increment
isomorphism. Consider the part of $\pi^{e_i}$
that stays in $\cup_{b=c}^{b=i-1}Q^{e_i}_{I_b}$.  Takes two states
$q^{e_i}_{l}$ $\in$ $Q_{I_{l}}^{e_i}$ and $q^{e_i}_{l+1}$ $\in$
$Q_{I_{l+u}}^{e_i}$, such that $q^{e_i}_{l+1} =
\delta(w(l+1),q^{e_i}_{l})$, and let $q^{e_*}_{l}$ $\in$
$Q^{e_*}_{I_{0}}$ be state corresponding to $q^{e_i}_{l}$ $\in$
$\pi^{e_*}$. By construction, there exists
$q_{l+1}^{e_*}=\delta^{e_*}(q_l^{e_*},(w(l+1),u))$, and
$q_{l+1}^{e_*}\in Q_{I_{0}COPY}^{e_*}$. This state is the state
corresponding to $q_{l+1}^{e_i}$ by the increment isomorphism. Let
$q_k^{e_i}$ $\in$ $Q_{I_{z<i}}^{e_i}$ be the last state of $\pi^{e_i}$
in $\cup_{b=c}^{b=i-1}Q^{e_i}_{I_b}$, and $q_k^{e_*}$ its
corresponding state in $Q_{I_{0}COPY}^{e_*}$. Let
$(w(1),c_1)(w(2),c_2){\dots}(w(k),c_k)$ be the part of $w_c$ that has
been read between $q_0^{e_*}$ and $q_k^{e_*}$.  We pose $s = \sum_{i =
1}^{i=k}c_k $; it is easy to see that $s = z$. Consider the state
$q_{k+1}^{e_i}=\delta^{e_i}(q_k^{e_i},w(k+1))$.  If $q_{k+1}^{e_i}$
$\in$ $Q_{I_{l>i}}^{e_i}$, there exists a transition
$(q^{e_i}_k,(w(k+1),q_{k+1}^{e_i})$ $\in$ $\delta^{e_i}$ with
$q_{k+1}$ $\in$ $Q_{I_{i+l}}^{e_i}$. Due to the communication
equivalence property, there exists a transition
$(q^{e_*}_{k},(w(k+1),i-z),q^{e_*}_{k+1})$ $\in$ $\delta^{e_*}$ with
$q^{e_*}_{k+1}$ the state isomorphic to $q^{e_i}_k$ in
$Q_{I_{l}}^{e_0}$. Due to the forward equivalence between
$Q_{I_{i+l}}^{e_i}$ and $Q_{I_{l}}^{e_0}$, the result holds.  If
$q_{k+1}^{e_i},sc^{e_i}$ $\in$ $Q_{I_{i}}^{e_i}$ then, by
construction, there exists
$q^{e_*}_{k+1}=\delta^{e_*}(q^{e_*}_{k},(w(k+1),i-z-1))$ and
$q^{e_*}_{k+1}\in Q_{I_{1}}^{e_*}$. This state is the state
corresponding to $q^{e_i}_k$ by the increment isomorphism. Due to the
isomorphism relation between $Q_{I_{i}}^{e_i}$ and $Q_{I_{1}}^{e_*}$,
the result holds.
\end{itemize}
\end{proof}
